# Supplementary material for: Self-assembly of dodecagonal and octagonal quasicrystals in hard spheres on a plane
Source: arXiv:2202.12726 ancillary file (2022-02-25)
Supplement: Supplementary file 1 [file SI.pdf]

# Non-additive self-assembly and quasicrystals – Supplemental Information

Etienne Fayen[1], Marianne Impéror-Clerc[1], Laura Filion[2], Giuseppe Foffi [1], Frank Smallenburg[1]
[1] *Université Paris-Saclay, CNRS,*
*Laboratoire de Physique des Solides, 91405 Orsay, France*
[2] *Soft Condensed Matter,*
*Debye Institute of Nanomaterials Science,*
*Utrecht University, Utrecht, Netherlands*

## SIMULATION DETAILS

We perform a systematic exploration of parameter space for systems of $N = 2000$ particles, varying the composition $x_S$ between 0.05 and 0.95 in steps of 0.05 and the size ratio $q$ between 0.25 and 0.75 in steps of 0.05. The packing fraction $\eta$ ranged from 0.7 to up to 1.0 in steps of 0.01, where we only considered state points where the growing-particle simulations were able to rapidly reach the desired packing fraction without jamming. In other words, we assume that at packing fractions where jamming occurs during our initial compression, the system would likely be too densely packed to observe self-assembly on a reasonable time scale. Each self-assembly simulation is allowed to run for at least $10^6 \tau_{\mathrm{MD}}$, with $\tau_{\mathrm{MD}} = \sqrt{m\sigma_L^2/k_B T}$ our simulation time unit, $m$ the mass of a particle (chosen equal for both species), $\sigma_L$ the large-particle diameter, and $k_B$ Boltzmann's constant. Subsequently, longer simulations were performed for state points where self-assembly was considered likely to occur on a reasonable time-scale based on the final pressure of the first simulations. In particular, we extended the simulations at state points with a pressure $16 \lesssim P\sigma_A^2/k_B T \lesssim 33$ to a total length of $5 \cdot 10^6 \tau_{\mathrm{MD}}$. Although this did not lead to a qualitative difference in the observed phase behavior, it allowed for some further annealing of some of the crystal phases, and increased the size of the observed patches of H2 crystal at the relevant state points.

For each simulation, we measured the two-dimensional structure factor of the final configuration using

$$S(\mathbf{k}) = \frac{1}{N} \left| \sum_{n=1}^{N} \exp(i\mathbf{k} \cdot \mathbf{r}_n) \right|^2 . \qquad (1)$$

where $\mathbf{k}$ is an allowed wave vector in the periodic simulation box, and $\mathbf{r}_n$ is the position of particle $n$.

The self-assembly of different phases was determined based on a visual inspection of the final configuration and the two-dimensional structure factor.

## FINAL CONFIGURATIONS

An archive of final configurations for the data set depicted in Figure 3 of the main text is provided as supplemental data for this manuscript. In particular, we provide a zipped archive of the final configurations, snapshot images, and diffraction patterns for all simulations performed using $N = 2000$ particles. The files are organized into folders and accompanied by HTML documents which allow for a rapid visualization of all simulation results for a single size ratio.

## $\mathrm{HEX_L}^+$ PHASE AT DIFFERENT COMPOSITIONS

As mentioned in the main text, we use the label $\mathrm{Hex_L}^+$ to refer to any phase consisting of a hexagonal lattice of large spheres interspersed with small spheres, regardless of the ordering of the smaller spheres. In Fig. 1, we show snapshots for a range of different compositions. The hexagonal symmetry of the large-sphere lattice remains in place even though the concentration of small spheres varies drastically. For low compositions $x_S$, only a few small spheres are randomly interspersed in the triangular holes in the lattice. This concentration increases all the way up to $x_S \simeq 2/3$, at which point all triangular holes in the lattice are filled, corresponding to the T1 crystal phase. Above this concentration, the large particles start to become more separated, as additional small particles fill the gaps between them. While this leads to local lattice distortions and a decrease in hexagonal ordering (e.g. at $x_S = 0.7$), overall the system maintains its hexagonal symmetry. In principle, pushing these systems to larger packing fractions may stabilize more ordered phases, such as those predicted by the infinite-pressure phase diagram in the main text.

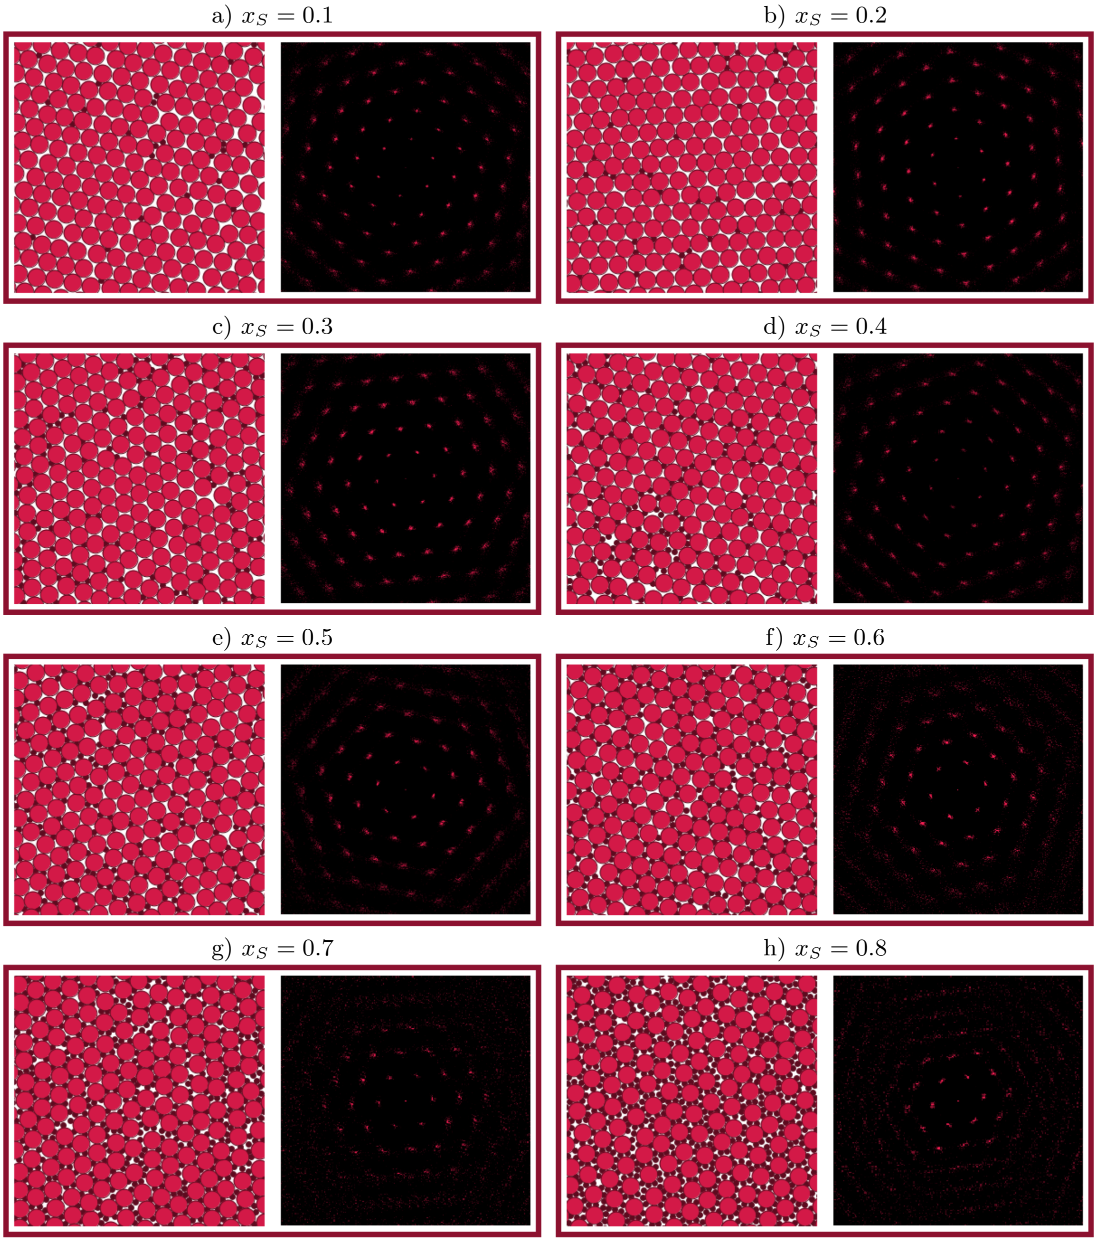


FIG. 1: Variations of the $\mathrm{Hex_L}^+$ phase, at size ratio $q = 0.35$ and varying compositions $x_S$. The packing fractions for the snapshots vary from $\eta = 0.82$ in (a) to $\eta = 0.96$ in (h), in steps of 0.02.

However, these high-density phases are likely hard to reach via spontaneous self-assembly due to the kinetic arrest that occurs at high packing fractions.

## TILING ANALYSIS

As mentioned in the main Method section, tiles are reconstructed from the simulation snapshots by identifying cycles in the network of large particles neighbours. We consider that two large particles are neighbours if they are separated by a distance smaller than $1.7\sigma_{LL}$. Since this cutoff distance is larger than $\sqrt{2}\sigma_{LL}$, crossing bonds are formed inside small S1 squares. We remove those crossing bonds before further analysis.

To characterise the neighbour network, we compute the bonds length and angle distributions, as shown in Figure 2. Bond angles are relative to the horizontal. In the vicinity of the QC8 region, the bond length distribution is clearly

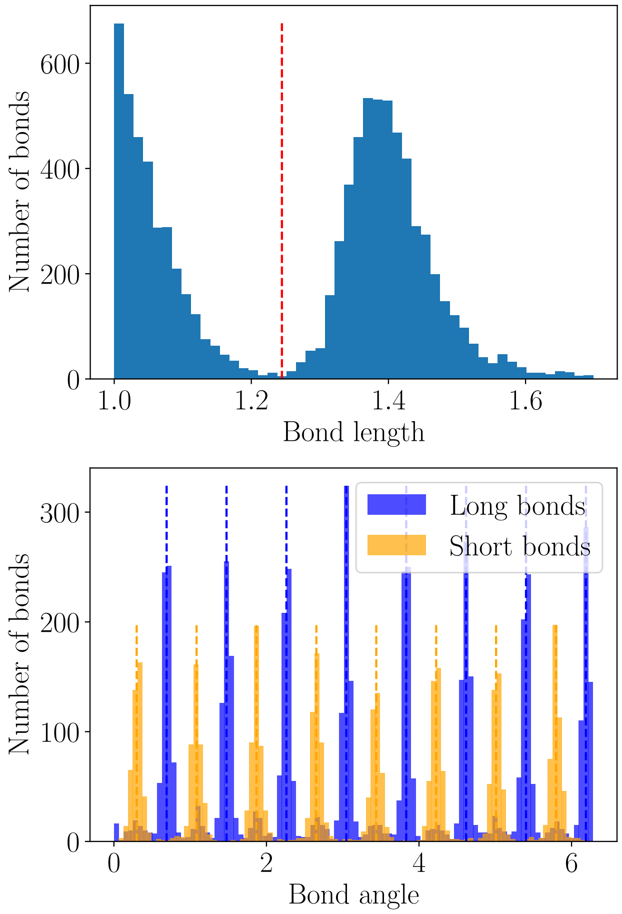


FIG. 2: Neighbour bonds characterisation in a system of $10^4$ non-additive hard disks, with size ratio $q = 0.5$, composition $x_S = 0.675$ and packing fraction $\eta = 0.86$. This system forms an octagonal random tiling quasicrystal, as shown in Figure 4 of the main text. (Top) Bonds length distribution showing a clear distinction between short and long populations. The vertical red line highlights the cutoff value obtained as the minimum in the dip. (Bottom) Bond angle distribution. The 16 peaks correspond to the possible edge orientations in the tiling underlying the reported octagonal quasicrystal. Short t(orange) and long (blue) bond follow two distinct set of 8 orientations, offset by $\pi/8$.

bimodal. A cutoff is set at the minimum of the distribution in-between the two peaks, which discriminates between long and short bonds. Since the cutoff value can vary slightly with the composition and packing fraction of the system, we determine it separately for each snapshot. The bond angle distribution exhibits 16 sharp peaks centered on the directions of an ideal tiling of large squares, small squares and equilateral triangles. Correlating the orientation with the bond length shows that short and long bonds each follow a distinct set of 8 orientations, offset by $\pi/8$.

## LIFT TO FOUR DIMENSIONS

For the square-triangle tiling associated with the QC12 phase, it is well known that global twelve-fold symmetry only occurs under the condition that the two area fractions of the tiling covered by squares and triangles are the same and equal to 1/2 [1, 2]. Here, we determine under what conditions the QC8 phase can exhibit 8-fold symmetry. To this end, we consider a QC8 tiling consisting of large squares $S$, small squares $s$, and triangles $T$, with long edge length $a$. Counting the different orientations, this results in a total of 12 different tiles: two orientations of both types of squares, and 8 orientations of the triangles. These are listed in Table I. We then consider an infinite, globally uniform[2] tiling consisting of a mixture of these tiles, with the area fraction covered by each tile type denoted as $\Sigma_i$ for the large squares, $\sigma_i$ for the small squares, and $\tau_i$ for the triangles, where $i$ denotes the orientation of the tile.

The first obvious constraint on our tiling is that it should cover the entire plane. Hence, the area fractions must

| Name | Tile | Area $A_{X_i}$ | Hyperslope $B_{X_i}$ | $\det B_{X_i}$ |
|---|---|---|---|---|
| $S_1$ | 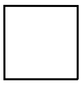 | $a^2$ | $\begin{pmatrix} 1 & 0 \\ 0 & -1 \end{pmatrix}$ | -1 |
| $S_2$ | 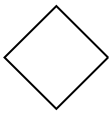 | $a^2$ | $\begin{pmatrix} -1 & 0 \\ 0 & 1 \end{pmatrix}$ | -1 |
| $s_1$ | 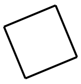 | $(2-\sqrt{2})a^2$ | $(1+\sqrt{2})\begin{pmatrix} 0 & -1 \\ -1 & 0 \end{pmatrix}$ | $-3-2\sqrt{2}$ |
| $s_2$ | 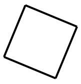 | $(2-\sqrt{2})a^2$ | $(1+\sqrt{2})\begin{pmatrix} 0 & 1 \\ 1 & 0 \end{pmatrix}$ | $-3-2\sqrt{2}$ |
| $T_{1,5}$ | 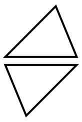 | $\frac{1}{2\sqrt{2}}a^2$ | $\begin{pmatrix} 1 & -2 \\ 0 & 1 \end{pmatrix}$ | 1 |
| $T_{2,6}$ | 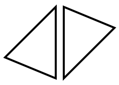 | $\frac{1}{2\sqrt{2}}a^2$ | $\begin{pmatrix} -1 & 0 \\ 2 & -1 \end{pmatrix}$ | 1 |
| $T_{3,7}$ | 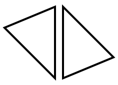 | $\frac{1}{2\sqrt{2}}a^2$ | $\begin{pmatrix} -1 & 0 \\ -2 & -1 \end{pmatrix}$ | 1 |
| $T_{4,8}$ | 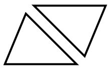 | $\frac{1}{2\sqrt{2}}a^2$ | $\begin{pmatrix} 1 & 2 \\ 0 & 1 \end{pmatrix}$ | 1 |

TABLE I: Summary of the 12 different tiles comprising the QC8 tiling. The third column reports the area of each tile, assuming that large squares have edges of length $a$. The fourth column contains the constant hyperslope of each tile, *i.e.* the 2x2 matrix that maps points inside that tile in the original tiling to the perpendicular space. The last column displays the determinant of the hyperslope for each tile, which is used to obtain Eq 7.

satisfy

$$\Sigma + \sigma + \tau = 1, \tag{2}$$

where $\Sigma = \sum_i \Sigma_i$, $\sigma = \sum_i \sigma_i$, and $\tau = \sum_i \tau_i$.

One set of constraints on these tile concentrations follows from the simple observation that each edge must have an opposing partner. Considering, for example, the short edge in triangle $T_1$, this leads to the constraint that

$$n_{T_1} + n_{s_1} = n_{T_5} + n_{s_1}, \tag{3}$$

with $n_{X_i}$ denotes the number of tiles of type $X_i$. This trivially implies that $\tau_1 = \tau_5 = \tau_{15}/2$, and likewise it can be shown that $\tau_2 = \tau_6 = \tau_{26}/2$, $\tau_3 = \tau_7 = \tau_{37}/2$, and $\tau_4 = \tau_8 = \tau_{48}/2$.

Another constraint on the various tile concentrations can be obtained by lifting the tiling to four-dimensional space. For this, we follow the procedure outlined in e.g. [1–3]. In particular, in the QC8 tiling, each long edge can only lie along one of 4 different orientations $\mathbf{e}_1$ through $\mathbf{e}_4$, illustrated in Fig. 3(left). Short edges can then be constructed by taking the difference between two of these vectors (e.g. $\mathbf{e}_2 - \mathbf{e_1}$). As a result, each vertex in our tiling can be written as a linear combination of an integer number of the four vectors $\mathbf{e}_i$, and hence can be seen as a point on a four-dimensional lattice. We then associate each vector $\mathbf{e}_i$ with a corresponding vector $\mathbf{e}_i^\perp$, illustrated in Fig. 3(right), such that each vertex in the tiling can be uniquely associated with a point in the perpendicular space [3, 4].

We can then consider a mapping $\phi(\mathbf{r})$ that maps each vertex in our original tiling to its corresponding point in the perpendicular space. Within each tile, $\phi(\mathbf{r})$ is a linear interpolation between the mapped vertices of that tile. Hence, $\phi$ is a continuous, piecewise linear function, with a constant hyperslope within each tile. The hyperslope within one

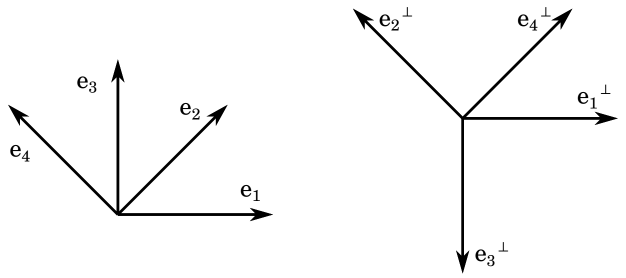


FIG. 3: Projections of the 4D lift vectors on the parallel (Left) and perpendicular (Right) sub-spaces.

tile is completely determined by the vectors that form it. Hence, tiles of the same type and orientation have the same hyperslope. Specifically, within a tile $X_i$, the hyperslope $B_{X_i}$ is given by:

$$B_{X_i} = \begin{pmatrix} \frac{\partial \phi_x}{\partial x} & \frac{\partial \phi_x}{\partial y} \\ \frac{\partial \phi_y}{\partial x} & \frac{\partial \phi_y}{\partial y} \end{pmatrix}. \tag{4}$$

In Table I, we report the hyperslope for each of the 12 tiles in the QC8 tiling.

In a globally uniform tiling, over long distances $\mathbf{r}$, $\phi(\mathbf{r})$ has a well-defined average hyperslope $B$, which can be written as the weighted sum of the hyperslopes of the individual tiles [2]:

$$B = \sum_{i=1}^{2} \Sigma_i B_{S_i} + \sum_{i=1}^{2} \sigma_i B_{s_i} + \sum_{i=1}^{8} \tau_i B_{T_i}. \tag{5}$$

Following Ref. [2], uniformity of the tiling then imposes that

$$\sum_{i=1}^{2} \Sigma_i \det B_{S_i} + \sum_{i=1}^{2} \sigma_i \det B_{s_i} + \sum_{i=1}^{8} \tau_i \det B_{T_i} = \det B. \tag{6}$$

Using the matrices listed in Table I, this leads to the following constraint:

$$\Sigma + (3+2\sqrt{2})\sigma - \tau = (\Sigma_1 - \Sigma_2)^2 + (3+2\sqrt{2})(\sigma_1 - \sigma_2)^2 - \tau^2 + (2+2\sqrt{2})(\tau_{15} - \tau_{26} + \tau_{37} - \tau_{48})(\sigma_1 - \sigma_2) + 8(\tau_{15}\tau_{37} + \tau_{26}\tau_{48}). \tag{7}$$

This constraint can be regarded as the equivalent of the Nienhuis relation [2, 5] for the (QC12) square-triangle tiling, but for our QC8 tiling.

For a maximally symmetric tiling with eight-fold symmetry, the requirement is that all orientations of each tile appear in the same amount [2]. In other words:

$$\Sigma_1 = \Sigma_2 = \frac{\Sigma}{2} \tag{8}$$

$$\sigma_1 = \sigma_2 = \frac{\sigma}{2} \tag{9}$$

$$\tau_{15} = \tau_{26} = \tau_{37} = \tau_{48} = \frac{\tau}{4}. \tag{10}$$

When we impose this, the average hyperslope $B$ vanishes, and as a result the right-hand side of Eq. 7 similarly becomes zero, yielding:

$$\Sigma + (3 + 2\sqrt{2})\sigma - \tau = 0. \tag{11}$$

Finally, we can express the area fractions $\Sigma$, $\sigma$ and $\tau$ in terms of the particle composition $x_S$ by using the known composition of each tile, combined with equations 2 and 11 (see equations 3, 4 and 5 of the main text).

**References**

[1] Oxborrow, M. & Henley, C. L. Random square-triangle tilings: A model for twelvefold-symmetric quasicrystals. *Physical Review B* **48**, 6966 (1993).

[2] Impéror-Clerc, M., Jagannathan, A., Kalugin, P. & Sadoc, J.-F. Square-triangle tilings: an infinite playground for soft matter. *Soft Matter* **17**, 9560–9575 (2021).

[3] Baake, M., Ecija, D. & Grimm, U. A guide to lifting aperiodic structures. *Zeitschrift für Kristallographie-Crystalline Materials* **231**, 507–515 (2016).

[4] Zu, M., Tan, P. & Xu, N. Forming quasicrystals by monodisperse soft core particles. *Nature Communications* **8**, 1–9 (2017).

[5] Nienhuis, B. Exact solution of random tiling models. *Physics Reports* **301**, 271–292 (1998).
